# Supplementary material for: Modeling Insights from COVID-19 Incidence Data: Part I -- Comparing COVID-19 Cases Between Different-Sized Populations
Source: arXiv:2211.09010 ancillary file (2022-11-14)
Supplement: Supplementary file 1 [file Covid_Cluster_Paper_Supplement__1_.pdf]

# Supplementary Materials

Ryan Wilkinson* and Marcus Roper†

*University of California, Los Angeles Department of Mathematics*

(Dated: November 14, 2022)

## SI. ISOLATING EARLY AND LATE CASE CURVE PHASES

To identify which sections of cumulative case curves corresponded to surges, we first pre-processed data from The COVID Tracking Project[1] to estimate the instantaneous number of infected individuals in each State. Instantaneous case numbers were estimated by assuming that each new measured case was reported 5 days after actual infection occurred, and then modeling the length of time each individual was infected with a seven day delayed exponential decay curve that assumed half of infected individuals would no longer be infectious after fourteen days (Fig S2). Then, the beginning and end of the first and final concave peak in the resulting infectious curves were recorded, and the cumulative case curve associated with these two peaks was isolated (Table S1). The first (early) phase occurs at the beginning of each State's outbreak without exception, and the final (late) phase in the data used occurs usually around the period of the Thanksgiving and Christmas Holiday season, sometimes extending into January of 2021.

## SII. CLUSTERING EARLY AND LATE CASE CURVE PHASES

To cluster our isolated phase case curves, we first devised a metric for computing dissimilarity or distance between phases. To account for differences in scale that are expected between states of different population sizes as well as to account for differences in onset of the waves due to different times of first COVID introduction to the State, or differences in the timing of public health measures such as Stay at Home orders or school closures, we measured the residual dissimilarity between each pair of curves after they had been aligned. Mathematically, this calculation amounts to defining a dissimilarity function $f(\mathbf{X}, \mathbf{Y}, T, S)$ for two time series $\mathbf{X}$ and $\mathbf{Y}$ given a shift in time $T$ and shift in scale $S$

$$f(\mathbf{X}, \mathbf{Y}, T, S) = \begin{cases} \frac{1}{\ell(\mathbf{X})} \sum_{i=1}^{\ell(\mathbf{X})} \left( \log\left(X(i)\right) - \left(\log(Y(i-T)) + S\right)\right)^2 & , \quad \ell(\mathbf{X})/\ell(\mathbf{Y}) \notin (0.5, 2) \\ \infty & , \quad \text{otherwise} \end{cases} \tag{S1}$$

---

* https://www.math.ucla.edu/~rwilkinson/

† https://www.marcusroper.org/

where $\ell(\mathbf{X})$ is the number of time points recorded in the time series $\mathbf{X}$. The $\infty$ is here included so as to invalidate the comparison of two states where one State's surge length is over double the other's. The final dissimilarity metric was then constructed via minimizing this function applied to both the cumulative data and the daily data over $T$ and $S$ for every pair of states, i.e. if $\mathbf{X}_i$ is the $i$th State surge, then the dissimilarity between surge $i$ and $j$ is

$$d_{ij} = \min_{(T,S)\in\mathcal{T}} \left\{ f(\mathbf{X}_i, \mathbf{X}_j) + f\big(\text{diff}(\mathbf{X}_i), \text{diff}(\mathbf{X}_j)\big) \right\} \tag{S2}$$

Here $\mathcal{T}$ is the set of pairs $(S,T)$ such that $T$ is an integer where shifting a time series to the right by $T$ satisfies the property that 80% of the smallest curve's length overlaps with the other curve after shifting, and $\text{diff}(\mathbf{X})$ is a discrete derivative;

$$\text{diff}(\mathbf{X})_i = \begin{cases} 0 & , \quad i = 1 \\ \mathbf{X}_i - \mathbf{X}_{i-1} & , \quad i > 1 \end{cases} \tag{S3}$$

Such a minimization attempts to match two surges' values and derivatives as closely as possible.

$d_{ij}$ was computed for every pair of U.S. states including the District of Columbia to generate a set of pairwise distances which was used to cluster. The WPGMA algorithm [2] was then performed on these pairwise distances to cluster phases together, where the number of clusters was chosen heuristically by finding an "elbow" on the curve generated from plotting the number of clusters versus the cutoff distance (Fig. S1). We then curated the clusters and manually combined suitable clusters together when such combinations maintained curve homology, and excluded two curves that did not cluster well with any other curve (Florida and Arizona late phase). Additionally $s_{ij}$, the minimizing $S$ value of the function $f$ (i.e. the upwards or downwards shift in the curves on the log scale), was stored, and is used later in section IIB as a measure of the scale difference between COVID-contracting populations of each State. Specifically, our estimated ratio of COVID-contracting populations between State $i$ and State $j$ is given by $e^{s_{ij}}$.

## SIII. CORRELATING CLUSTERING WITH OTHER VARIABLES

We look for explanatory variables than can elucidate similarities between State case curves within clusters. These variables may be either categorical (whether neighboring states or political party of the governor correlate to clustering, or whether states tended to stay clustered throughout the pandemic) or numerical (whether population centroid differences, Trump voting percentage differences, testing positivity rates, or school reopening times correlate to clustering). We use permutation tests to calculate $p$ values against these variables explaining the observed clustering. For variables dealing with pairwise relations, we performed a modified Mantel test, which correlates our dissimilarity metric $d_{ij}$ with the pairwise relation at hand. We restrict permutations to occur only within clusters as opposed to over the entire data set since the scales of dissimilarity scores are meaningful only in the cases where the curves being

compared have similar shape, i.e. curves that are in the same cluster. For data that we did not interpret as pairwise or whose relation to our clustering was not readily measured via correlation, we devised a statistic to measure the performance of our clustering with regard to the variable in question and tested it against 50,000 permutations of the clustering IDs. The statistic tested depended on the variable at hand. To test our clustering against the political party of the governors of each state in the cluster, we first computed the percentage of governors in each cluster belonging to the most represented party in the cluster (for example, a hypothetical cluster with five Democratic governors and three Republican governors would be measured as 5/8). We then measured our statistic of the overall clustering to be the average of these percentages across all clusters. To measure whether our clustering tended to group certain states together both in the early phase and later phase of the pandemic, we computed the average percentage of pairs of states in each cluster that were clustered together in both early phase and late phase. For testing whether neighboring states tended to be clustered together, we computed the average percentage of states in each cluster who shared a neighbor in the cluster. To test whether our clustering was influenced by school reopening times or testing positivity rates, we computed the average variance of these variables over all clusters. A summary of the statistics used can be found in table II. For all of these tests, the $p$ value reported in table II refers to the fraction of random permutations that yielded a higher statistic than that of the actual clustering.

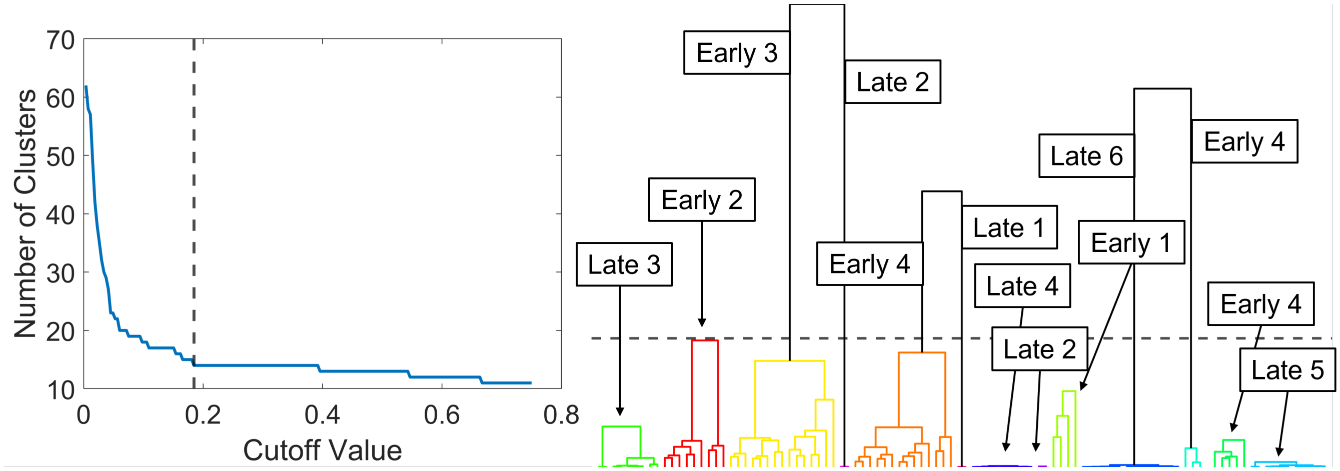


FIG. S1. Left: the number of clusters identified is plotted against the distance used by the WPGMA algorithm [2] to differentiate different subtrees on the dendrogram. The vertical dotted line represents a point at which raising the cutoff value no longer decreases the number of clusters by an appreciable amount. Right: the dendrogram. The black dotted line represents the chosen cutoff value corresponding to the left pane. Different subgroups representing the 14 uncurated clusters are shown in different colors. The cluster labels both early and late are indicated with the boxes and arrows on the dendrogram.

## SIV. ESTIMATING CURRENT INFECTIOUS FROM CUMULATIVE CASE DATA

In order to determine when Covid surges took place, we first needed some way of estimating how many individuals were currently infected day by day from cumulative data. To this end, we first determined the number of new cases recorded per day via differencing (described in Eq. 3 of the main paper). We then assumed that, on average, individuals remained infected for at least seven days, and thereafter this number decreased to one eighth exponentially for an

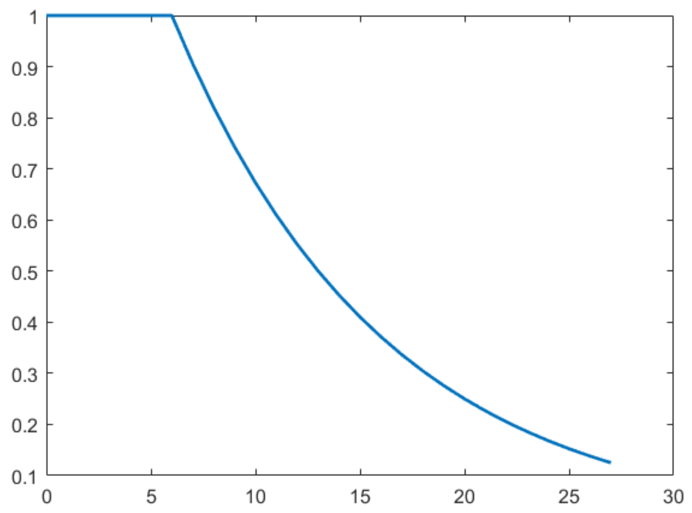


FIG. S2. The assumed remaining fraction of people who are still infected if their infection started $x$ days ago, where $x$ is the horizontal axis.

additional three weeks, and then immediately to 0 (Fig. S2). We then assumed that there was a five day reporting delay between becoming infected and testing positive, although the exact timing of this reporting delay didn't seem to affect the qualitative behavior of the resulting estimated curve, nor did adjusting the assumption of how long individuals were infected. This is a simplistic and relatively ad hoc way of determining the current infectious numbers, and is less precise than more complex methods, but has the benefit of making very few modeling assumptions beyond anecdotal observations on Covid recovery times. The nature of the clustering technique employed in this paper required very little precision, so this method detracts little from our process.

## SV. SPLITTING DATA INTO EARLY AND LATE SURGES

Armed with estimated current infectious curves for each state's data, we then defined a Covid "surge" in our context to be a period of exponential growth followed by a plateau and sudden drop off (Fig. S3). This definition was made after a considerable amount of trial and error in the clustering that followed different, specific surge definitions. Using this plateau definition, the beginning and end of each surge for each state was identified. Since all states had a surge at the beginning of the pandemic (March 2020 for our data) and around Christmas or Thanksgiving of 2020, we considered only these surges for consistency. See table S1.

## SVI. FITTING AN SIR CURVE TO CASE DATA

There are many statistical methods to estimate parameters from data ([3–5], to name just a few). These often rely on assuming underlying distributions for errors in both the assumed model and the data. To reflect a complete ignorance of error distributions for the model and a lack of confidence in the data given, we opted for a simple approach. We derived the model parameters which produced the curve that fit the data well in a least-squares sense

| State Name | First Wave | Last Wave |
|---|---|---|
| AK | 19-Mar-2020 to 19-Mar-2020 | 18-Sep-2020 to 21-Dec-2020 |
| AL | 15-Mar-2020 to 15-Mar-2020 | 21-Oct-2020 to 15-Feb-2021 |
| AR | 14-Mar-2020 to 14-Mar-2020 | 27-Oct-2020 to 30-Jan-2021 |
| AZ | 14-Mar-2020 to 14-Mar-2020 | 30-Sep-2020 to 05-Feb-2021 |
| CA | 04-Mar-2020 to 04-Mar-2020 | 31-Oct-2020 to 05-Feb-2021 |
| CO | 09-Mar-2020 to 09-Mar-2020 | 03-Oct-2020 to 23-Dec-2020 |
| CT | 14-Mar-2020 to 14-Mar-2020 | 05-Oct-2020 to 27-Dec-2020 |
| DC | 12-Mar-2020 to 12-Mar-2020 | 31-Oct-2020 to 05-Feb-2021 |
| DE | 17-Mar-2020 to 17-Mar-2020 | 31-Oct-2020 to 30-Jan-2021 |
| FL | 08-Mar-2020 to 08-Mar-2020 | 17-Oct-2020 to 25-Dec-2020 |
| GA | 09-Mar-2020 to 09-Mar-2020 | 25-Nov-2020 to 12-Feb-2021 |
| HI | 17-Mar-2020 to 17-Mar-2020 | 26-Dec-2020 to 09-Feb-2021 |
| IA | 11-Mar-2020 to 11-Mar-2020 | 24-Oct-2020 to 14-Dec-2020 |
| ID | 19-Mar-2020 to 19-Mar-2020 | 17-Sep-2020 to 28-Dec-2020 |
| IL | 10-Mar-2020 to 10-Mar-2020 | 05-Oct-2020 to 27-Dec-2020 |
| IN | 11-Mar-2020 to 11-Mar-2020 | 30-Sep-2020 to 29-Dec-2020 |
| KS | 16-Mar-2020 to 16-Mar-2020 | 21-Oct-2020 to 18-Dec-2020 |
| KY | 13-Mar-2020 to 13-Mar-2020 | 14-Oct-2020 to 22-Dec-2020 |
| LA | 12-Mar-2020 to 12-Mar-2020 | 05-Nov-2020 to 24-Dec-2020 |
| MD | 12-Mar-2020 to 12-Mar-2020 | 30-Oct-2020 to 01-Feb-2021 |
| ME | 16-Mar-2020 to 16-Mar-2020 | 20-Oct-2020 to 04-Feb-2021 |
| MI | 01-Mar-2020 to 01-Mar-2020 | 04-Oct-2020 to 27-Dec-2020 |
| MN | 10-Mar-2020 to 10-Mar-2020 | 21-Oct-2020 to 22-Dec-2020 |
| MO | 18-Mar-2020 to 18-Mar-2020 | 29-Oct-2020 to 23-Dec-2020 |
| MS | 15-Mar-2020 to 15-Mar-2020 | 30-Oct-2020 to 08-Feb-2021 |
| MT | 18-Mar-2020 to 18-Mar-2020 | 15-Sep-2020 to 25-Dec-2020 |
| NC | 12-Mar-2020 to 12-Mar-2020 | 27-Sep-2020 to 17-Feb-2021 |
| ND | 19-Mar-2020 to 19-Mar-2020 | 14-Aug-2020 to 18-Dec-2020 |
| NE | 12-Mar-2020 to 12-Mar-2020 | 09-Sep-2020 to 22-Dec-2020 |
| NH | 15-Mar-2020 to 15-Mar-2020 | 28-Oct-2020 to 08-Feb-2021 |
| NJ | 09-Mar-2020 to 09-Mar-2020 | 18-Sep-2020 to 12-Feb-2021 |
| NM | 12-Mar-2020 to 12-Mar-2020 | 20-Sep-2020 to 22-Dec-2020 |
| NV | 12-Mar-2020 to 12-Mar-2020 | 24-Sep-2020 to 04-Feb-2021 |
| NY | 06-Mar-2020 to 06-Mar-2020 | 28-Oct-2020 to 15-Feb-2021 |
| OH | 13-Mar-2020 to 13-Mar-2020 | 09-Oct-2020 to 29-Jan-2021 |
| OK | 16-Mar-2020 to 16-Mar-2020 | 01-Nov-2020 to 09-Feb-2021 |
| OR | 09-Mar-2020 to 09-Mar-2020 | 26-Oct-2020 to 24-Jan-2021 |
| PA | 09-Mar-2020 to 09-Mar-2020 | 27-Sep-2020 to 24-Jan-2021 |
| RI | 12-Mar-2020 to 12-Mar-2020 | 26-Sep-2020 to 26-Jan-2021 |
| SC | 12-Mar-2020 to 12-Mar-2020 | 25-Nov-2020 to 17-Feb-2021 |
| SD | 16-Mar-2020 to 16-Mar-2020 | 11-Sep-2020 to 24-Dec-2020 |
| TN | 12-Mar-2020 to 12-Mar-2020 | 30-Oct-2020 to 31-Jan-2021 |
| TX | 09-Mar-2020 to 09-Mar-2020 | 08-Nov-2020 to 14-Feb-2021 |
| UT | 15-Mar-2020 to 15-Mar-2020 | 20-Sep-2020 to 25-Dec-2020 |
| VA | 12-Mar-2020 to 12-Mar-2020 | 11-Oct-2020 to 16-Feb-2021 |
| VT | 16-Mar-2020 to 16-Mar-2020 | 15-Oct-2020 to 22-Dec-2020 |
| WA | 25-Feb-2020 to 25-Feb-2020 | 29-Oct-2020 to 08-Feb-2021 |
| WI | 13-Mar-2020 to 13-Mar-2020 | 05-Sep-2020 to 17-Sep-2020 |
| WV | 21-Mar-2020 to 21-Mar-2020 | 21-Oct-2020 to 08-Feb-2021 |
| WY | 17-Mar-2020 to 17-Mar-2020 | 08-Sep-2020 to 25-Dec-2020 |

TABLE S1. Estimates made for each surge time period from the analysis described in section SV

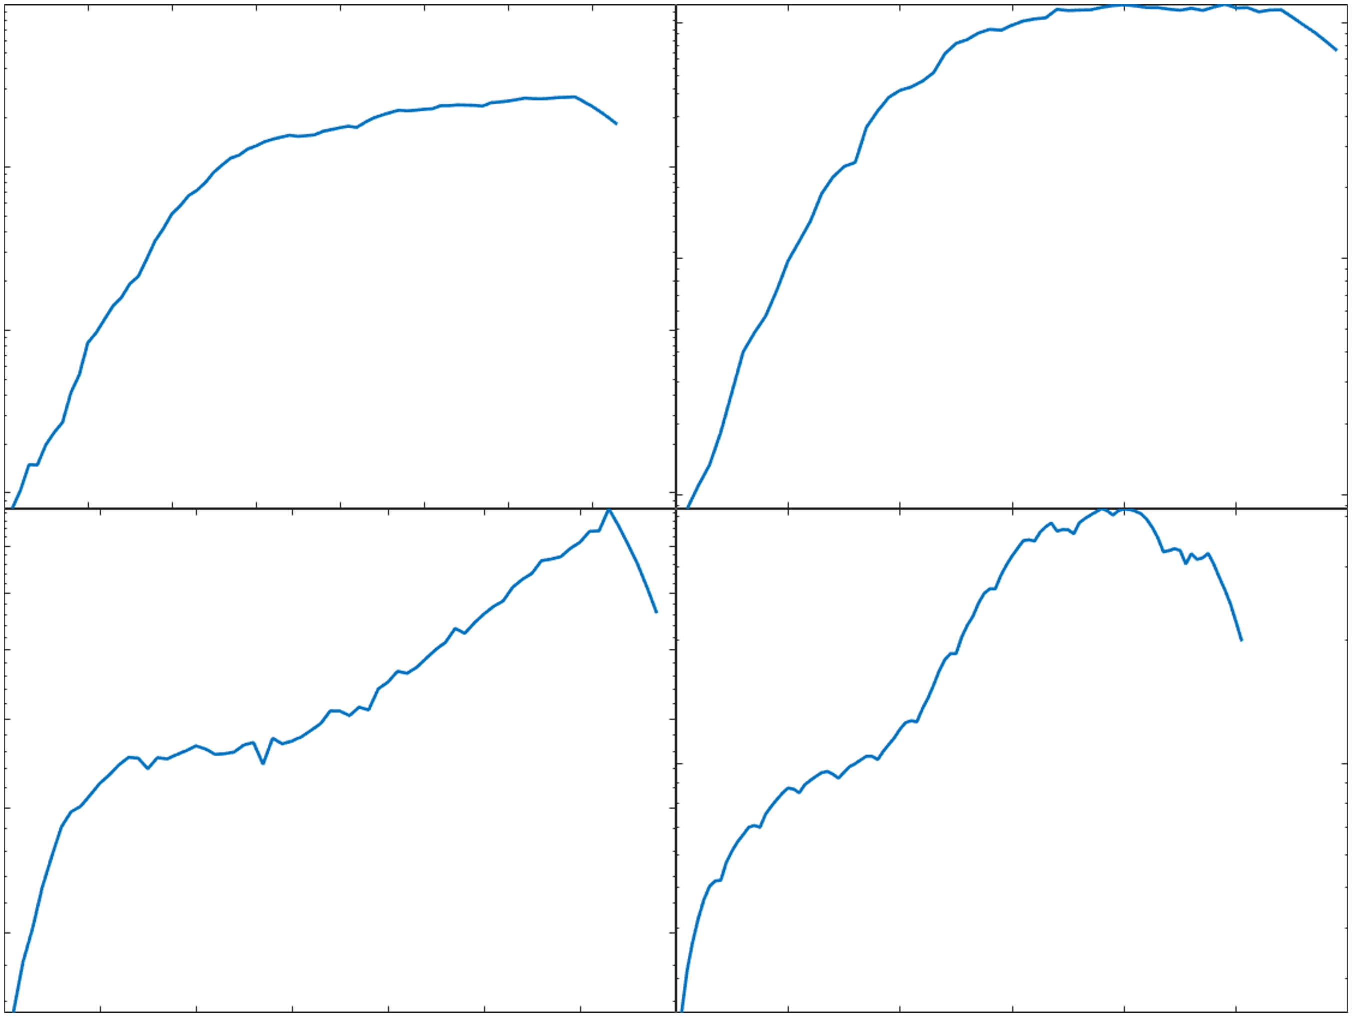

FIG. S3. Four examples of typical surges identified during the manual surge analysis. Top row: California and Georgia, early phase. Bottom row: Florida and Washington, late phase. Data shown are current infectious estimates (section SIV) shown on the log scale.

only. This objective is coincidentally equivalent to assuming Gaussian, time-independent error for the data, but was chosen mainly because minimizing least-squares error is a classical way of producing fits which "look" the best.

## SVII. THE PARAMETER ESTIMATION METHOD

Suppose we have a model $Y(t, \theta)$, where $t$ is a continuous variable and $\theta$ is a vector of parameters, and a set of time points $\{t_i\}$, $i = 1, 2, \ldots, n$, upon which data $X(t_i)$ are defined. Assume $Y$ and $X$ are vectors that are the same size. Fitting our model to the data means minimizing the following objective function

$$E(\theta) = \sum_{i=1}^{n} w_i ||Y(t_i, \theta) - X(t_i)||^2 \tag{S4}$$

for some set of weights $w_i$, whence the best-fitting parameter vector $\hat{\theta}$ may be written as

$$\hat{\theta} = \arg\min_{\theta} E(\theta) \tag{S5}$$

In this case, the model we desired to fit was the simple SIR model:

$$\begin{aligned}\frac{\mathbf{d}S}{\mathbf{d}t} &= -\beta SI/N_{tot} \\ \frac{\mathbf{d}I}{\mathbf{d}t} &= \beta SI/N_{tot} - \gamma I \\ \frac{\mathbf{d}R}{\mathbf{d}t} &= \gamma I\end{aligned} \tag{S6}$$

Since data was given in terms of cumulative cases, we have $Y(t, \theta) = I(t) + R(t)$, i.e. the number of people who are currently infected plus those that have been infected. In this case $\theta = (\beta, \gamma, N_{tot}, S(0), I(0))$. The model is differentiable with respect to $\theta$, so the minimum parameter vector may be found using gradient descent. Since the problem is non-convex, we optimized using many different initial guesses for $\theta$ in an effort to coax out the global minimum from many different local minima. In an effort to keep $\beta$ realistic, we also included constrained $\gamma$ to be between 0 and 1, since $\gamma$ (the disease removal rate) for Covid-19 can reasonably be assumed to be in that range, and almost certainly much smaller than 1. For best visual results such as those in the clustering analysis, we let $w_i = t_i^p$ and adjusted $p$ until the fit was to visual satisfaction.

---

[1] The Covid Tracking Project, `https://covidtracking.com/`.

[2] R. R. Sokal, A statistical method for evaluating systematic relationships., Univ. Kansas, Sci. Bull. **38**, 1409 (1958).

[3] R. E. Kalman, A new approach to linear filtering and prediction problems, Transactions of the ASME–Journal of Basic Engineering **82**, 35 (1960).

[4] I. J. Myung, Tutorial on maximum likelihood estimation, Journal of Mathematical Psychology **47**, 90 (2003).

[5] A. Doucet and A. M. Johansen, A tutorial on particle filtering and smoothing: Fifteen years later, Handbook of nonlinear filtering **12**, 3 (2009).
